# Supplementary material for: Coarse-grained Mori-Zwanzig dynamics in a time-non-local stationary-action framework
Source: arXiv:2202.10756 ancillary file (2022-09-25)
Supplement: Supplementary file 1 [file supp.pdf]

# Supporting Information for
## *Coarse-grained Mori-Zwanzig dynamics in a time-non-local stationary-action framework*


Piero Luchi,[1, 2, *] Roberto Menichetti,[1, 2, *] Gianluca Lattanzi,[1, 2] and Raffaello Potestio[1, 2, †]

[1] *Physics Department, University of Trento, via Sommarive, 14 I-38123 Trento, Italy*

[2] *INFN-TIFPA, Trento Institute for Fundamental Physics and Applications, I-38123 Trento, Italy*



(Dated: September 25, 2022)


This Supporting Information provides additional results that integrate those presented in the main text. Specifically, In Sec. I we report a brief summary of the Mori-Zwanzig formalism. In Sec. II we prove that the effective, time non-local coarse-grained (CG) action introduced in this work, when minimised with respect to the CG trajectory, results in the generalised Langevin equation (GLE) for the dynamics of the low-resolution system. In Sec. III we introduce a discretisation of the action that enables its calculation on the trajectory obtained by projecting the results of an atomistic molecular dynamics simulation of the system onto their CG counterpart. In Sec. IV we provide all the technical details regarding the minimisation of the discretised CG action aimed at extracting the optimised parameters of the GLE, explicitly discussing the constraints employed in the overall workflow. In Sec. V we derive the constraint that links the integral of the memory kernel to the diffusion coefficient. Finally, in Sec. VI we report the numerical integrator employed in this work to solve the GLE for the CG system.

### I. MORI-ZWANZIG FORMALISM

In principle, an arbitrary system composed by $n_A$ atoms can be simulated through the numerical integration of its Newton's equations of motion,

$$m_i \ddot{\mathbf{r}}_i = \mathbf{F}_i, \quad i = 1, ..., n_A, \\ \text{with} \quad \mathbf{F}_i = -\frac{\partial u(\boldsymbol{r})}{\partial \mathbf{r}_i}, \tag{1}$$

where $u(\boldsymbol{r}) = u_{\text{nb}}(\boldsymbol{r}) + u_{\text{bond}}(\boldsymbol{r})$ is the potential taking into account the non-bonded (van der Waals, electrostatic...) and bonded (bonds, angles, dihedrals...) interactions of the system, respectively. The numerical solution of these equations, although providing the most accurate results, is at present unmanageable for systems composed by a number of atoms that exceeds the hundreds of millions (provided that the cutting-edge computing technology is available, otherwise this upper bound decreases further). One thus needs to resort to a CG description: to this aim, we here review the Mori-Zwanzig (MZ) formalism.


* These authors contributed equally to this work.
† raffaello.potestio@unitn.it


The MZ formalism reformulates the dynamics of the system by virtue of a projection operator, and returns a generalized Langevin equation in which the motion of each CG degree of freedom is dictated by three separate terms. We here follow the approach by Hijòn *et al.* [1] and the systematic method described in Ref. [2], defining a projection operator on the Hilbert space of all possible choices of the CG variables, considering them as observables of the fine-grained system [3, 4].

We start by rewriting Eq. 1 in the form of Hamilton's equations for the atomistic system:

$$\frac{d\boldsymbol{\gamma}(t)}{dt} = \boldsymbol{\Lambda} \frac{\partial H(\boldsymbol{\gamma}(t))}{\partial \boldsymbol{\gamma}}, \tag{2}$$

where $\boldsymbol{\gamma} = (\boldsymbol{\gamma}_r, \boldsymbol{\gamma}_p) = (\mathbf{r}_1, \mathbf{r}_2, ..., \mathbf{r}_{n_A}, \mathbf{p}_1, \mathbf{p}_2, ..., \mathbf{p}_{n_A})$ contains the phase space coordinates of the $n_A$ atoms in the system, $H(\mathbf{p}, \mathbf{r})$ is the Hamiltonian, while

$$\boldsymbol{\Lambda} = \left( \begin{smallmatrix} \mathbf{0} & \mathbf{I} \\ -\mathbf{I} & \mathbf{0} \end{smallmatrix} \right)$$

is a symplectic matrix. We consider the vector of observables $\boldsymbol{\Gamma}(\boldsymbol{\gamma}) = (\mathbf{R}_1, \mathbf{R}_2, ..., \mathbf{R}_{N_B}, \mathbf{P}_1, \mathbf{P}_2, ..., \mathbf{P}_{N_B})$ corresponding to the phase space coordinates of $N_B$ pseudo atoms or *beads* in the CG system, which are functions of the phase space variables. Classical mechanics [5] allows one to rewrite the time evolution of the functions $\boldsymbol{\Gamma}$ as

$$\frac{d\boldsymbol{\Gamma}(\boldsymbol{\gamma}(t))}{dt} = L\boldsymbol{\Gamma}(\boldsymbol{\gamma}(t)), \\ \boldsymbol{\Gamma}(\boldsymbol{\gamma}(0)) = \boldsymbol{\Gamma}(\boldsymbol{\gamma}_0), \tag{3}$$

where we have defined the *Liouvillean* $L$

$$L = \sum_{i=1}^{n_A} \left( \frac{\partial H}{\partial \mathbf{p}_i} \cdot \frac{\partial}{\partial \mathbf{r}_i} - \frac{\partial H}{\partial \mathbf{r}_i} \cdot \frac{\partial}{\partial \mathbf{p}_i} \right). \tag{4}$$

Now, we use the MZ projection to map Eq. 3 onto the space of functions of CG variables, which is a subspace of the fine-grained observable space. The MZ projection is formally a conditional expectation with respect to the equilibrium distribution and it is defined, for a generic observable $\mathcal{O}(\boldsymbol{\gamma})$, as

$$P_{\boldsymbol{\Gamma}} \mathcal{O}(\boldsymbol{\gamma}) = \langle \mathcal{O} \rangle_{\boldsymbol{\Gamma}} = \mathbb{E}[\mathcal{O}|\boldsymbol{\Gamma}] = \\ = \frac{1}{\Omega(\boldsymbol{\Gamma})} \int \mathcal{O}(\boldsymbol{\gamma}') \delta(\boldsymbol{\Gamma}(\boldsymbol{\gamma}') - \boldsymbol{\Gamma}) \rho^{eq}(\boldsymbol{\gamma}') \mathrm{d}\boldsymbol{\gamma}', \tag{5}$$

with the normalisation factor

$$\Omega(\boldsymbol{\Gamma}) = \int \delta(\boldsymbol{\Gamma}(\boldsymbol{\gamma}') - \boldsymbol{\Gamma}) \rho^{eq}(\boldsymbol{\gamma}') d\boldsymbol{\gamma}' \tag{6}$$

and the canonical equilibrium distribution $\rho^{eq} = \frac{1}{Z}e^{-\beta H}$, where $Z$ is the canonical partition function.

After some manipulations, Eq. 3 can be recast in the form of the generalised Langevin equation (GLE) [2]:

$$\frac{d}{dt}\mathbf{\Gamma}(t) = L_P\mathbf{\Gamma}(t) - \int_0^t \mathcal{M}(\mathbf{\Gamma}(t-s),s)\frac{\partial}{\partial\mathbf{\Gamma}}\mathcal{S}(\mathbf{\Gamma}(t-s))ds + \beta^{-1}\int_0^t \frac{\partial}{\partial\mathbf{\Gamma}}\mathcal{M}(\mathbf{\Gamma}(t-s),s)ds + \boldsymbol{\mathcal{F}}_{\mathbf{\Gamma}}(t,\boldsymbol{\gamma}_0), \tag{7}$$

where

$$\mathcal{M}(\mathbf{\Gamma},t) = \beta P_{\mathbf{\Gamma}}([L_Q\mathbf{\Gamma}]\otimes[e^{tL_Q}L_Q\mathbf{\Gamma}]) \tag{8}$$

is the so-called friction matrix and is linked to the orthogonal dynamics, the term $\boldsymbol{\mathcal{F}}_{\mathbf{\Gamma}}(t,\boldsymbol{\gamma}_0)$ reads

$$\boldsymbol{\mathcal{F}}_{\mathbf{\Gamma}}(t,\boldsymbol{\gamma}_0) = e^{tL_Q}L_Q\mathbf{\Gamma}(\boldsymbol{\gamma}_0), \tag{9}$$

$Q_{\mathbf{\Gamma}} = I - P_{\mathbf{\Gamma}}$ is the orthogonal projection, and

$$\mathcal{S} = -\frac{1}{\beta}\ln(\Omega(\mathbf{\Gamma})) \tag{10}$$

is interpreted as a contribution to the free energy of the system.

Assuming now a fixed chemical structure for the system (no ongoing chemical reactions, and hence a fixed topology of bonded interactions), we define a mapping from the atomistic to the CG description:

$$\mathbf{R}_I = \mathbf{M}_I(\mathbf{r}) = \sum_{k\in S_I}\frac{m_k}{M_I}\mathbf{r}_k, \qquad \mathbf{P}_I = \Phi_I(\mathbf{p}) = \sum_{k\in S_I}\mathbf{p}_k, \tag{11}$$

where $\mathbf{R}_I$ and $M_I = \sum_{k\in S_I} m_k$ are the coordinates and the masses, respectively, of the $I^{th}$ CG bead, $I = 1,...,N_B$, $\mathbf{r}_k$ and $m_k$ the coordinates and the masses, respectively, of the $k^{th}$ atom, and $S_I$ is the set of atoms that map onto bead $I$. This explicit mapping together with further manipulations and simplifications (see again Refs. [1, 2, 6]) yields a more readable and computationally tractable form for the equations of motion of the CG system, namely

$$\frac{d\mathbf{R}_I}{dt} = \frac{\mathbf{P}_I}{M_I}, \qquad \frac{d\mathbf{P}_I}{dt} = -\frac{\partial U(\mathbf{R})}{\partial\mathbf{R}_I} - \int_0^t K(t-s)\frac{\mathbf{P}_I}{M_I}ds + \boldsymbol{\mathcal{F}}_I(t), \tag{12}$$

with $U$ being the effective potential of the CG configuration induced by the mapping, while $K(t-s)$ is defined as the memory kernel, here assumed to have no dependence on the coordinates of the CG pseudoparticles. In the following the function $\boldsymbol{\mathcal{F}}_I(t)$ describing the orthogonal dynamics, although in principle deterministic, will be identified with an autocorrelated noise linked to the memory kernel $K(t)$ via the fluctuation-dissipation theorem [7].

## II. DERIVATION OF THE GENERALISED LANGEVIN EQUATION VIA THE EXTREMISATION OF THE TIME NON-LOCAL ACTION FUNCTIONAL

In this Section we will prove that the time-non local action $\Sigma[\mathbf{R},\dot{\mathbf{R}};\boldsymbol{\zeta}]$ proposed in this work, with

$$\Sigma[\mathbf{R},\dot{\mathbf{R}};\boldsymbol{\zeta}] = \int_0^T dt\,\Big[K_R(\dot{\mathbf{R}}(t)) - U(\mathbf{R}(t)) + \sum_{J=1}^{N_B}\dot{\mathbf{R}}_J(t)\cdot\int_0^t dt'\,Q(t-t',\boldsymbol{\zeta})\dot{\mathbf{R}}_J(t') + \sum_{J=1}^{N_B}\boldsymbol{\xi}_J(t,\boldsymbol{\zeta})\cdot\mathbf{R}_J(t)\Big], \tag{13}$$

when plugged into the generalised Euler-Lagrange equation proposed by Ferialdi and Bassi [8],

$$\frac{\delta\Sigma[\mathbf{R},\dot{\mathbf{R}};\boldsymbol{\zeta}]}{\delta\mathbf{R}_I(s)} - \frac{d}{ds}\frac{\delta\Sigma[\mathbf{R},\dot{\mathbf{R}};\boldsymbol{\zeta}]}{\delta\dot{\mathbf{R}}_I(s)} = 0, \tag{14}$$

gives rise to the GLE for the dynamics of the $N_B$ particles in the CG system presented in Eq. 12, which we rewrite as

$$M\ddot{\mathbf{R}}_I(s) = \mathbf{F}_I(\mathbf{R}(s)) - \int_0^s dt' K(s-t',\boldsymbol{\zeta})\dot{\mathbf{R}}_I(t') + \boldsymbol{\xi}_I(s,\boldsymbol{\zeta}), \qquad \mathbf{F}_I(\mathbf{R}(s)) = -\frac{\partial U(\mathbf{R})}{\partial\mathbf{R}_I}\bigg|_{\mathbf{R}(s)}. \tag{15}$$

In Eq. 13-15, $(i)$ $K_R$ and $U$ are respectively the kinetic and potential energy of the CG particles, which are assumed to have the same mass $M$; $(ii)$ the memory kernel $K(\tau,\boldsymbol{\zeta})$ and the noise term[1] $\boldsymbol{\xi}_I(t,\boldsymbol{\zeta})$ are parametric functions of the properties $\boldsymbol{\zeta}$ that account for the effect of the fast variables, see the discussion in Sec. II of the main text, and satisfy the fluctuation-dissipation relation reported in Eq. 4 of the main text [7]; $(iii)$ $Q(\tau,\boldsymbol{\zeta})$ is a function whose time derivative is equal to the memory kernel, i.e. $\frac{d}{d\tau}Q(\tau,\boldsymbol{\zeta}) = K(\tau,\boldsymbol{\zeta})$; and $(iv)$ in Eq. 14 $\delta\Sigma/\delta\mathbf{R}_I(s)$ and $\delta\Sigma/\delta\dot{\mathbf{R}}_I(s)$ respectively represent functional derivatives of the action $\Sigma[\mathbf{R},\dot{\mathbf{R}};\boldsymbol{\zeta}]$ with respect to the positions and velocities of the $I$-th effective CG site at time $s\in[0,T]$.

We begin with the calculation of the positional functional derivative in Eq. 14: by performing this, one ob-

[1] As previously discussed, we are identifying with a stochastic force $\boldsymbol{\xi}_J(t,\boldsymbol{\zeta})$ what in our scheme should rather be a deterministic, fast-fluctuating term $\boldsymbol{\mathcal{F}}_J(t,\boldsymbol{\zeta})$ acting on each CG pseudoparticle as a consequence of the MZ projection, see Eqs. 9 and 12. In doing so, we are implicitly assuming that the two forces generate the same statistical properties as far as the CG system is concerned.

tains

$$\frac{\delta\Sigma}{\delta\mathbf{R}_I(s)} = \frac{\delta}{\delta\mathbf{R}_I(s)}\int_0^T dt\left[-U(\mathbf{R}(t)) + \sum_{J=1}^{N_B}\boldsymbol{\xi}_J(t,\boldsymbol{\zeta})\cdot\mathbf{R}_J(t)\right]$$
$$= \int_0^T dt\left[-\frac{\partial U(R)}{\partial\mathbf{R}_I}\bigg|_{\mathbf{R}(t)}\delta(s-t) + \boldsymbol{\xi}_I(t,\boldsymbol{\zeta})\delta(s-t)\right]$$
$$= -\frac{\partial U(\mathbf{R})}{\partial\mathbf{R_I}}\bigg|_{\mathbf{R}(s)} + \boldsymbol{\xi}_I(s,\boldsymbol{\zeta}), \quad (16)$$

where $\delta(s-t)$ is the Dirac delta function.

Let us now consider the velocity-dependent part, that is,

$$\frac{d}{ds}\frac{\delta\Sigma}{\delta\dot{\mathbf{R}}_I(s)} = \frac{d}{ds}\frac{\delta}{\delta\dot{\mathbf{R}}_I(s)}\sum_{J=1}^{N_B}\int_0^T dt\left[\frac{1}{2}M\dot{\mathbf{R}}_J^2(t) + \right.$$
$$\left. + \dot{\mathbf{R}}_J(t)\cdot\int_0^t dt'\; Q(t-t',\boldsymbol{\zeta})\dot{\mathbf{R}}_J(t')\right]. \quad (17)$$

The differentiation of the kinetic term is straightforward as in the position-dependent case, and results in

$$\frac{d}{ds}\frac{\delta}{\delta\dot{\mathbf{R}}_I(s)}\int_0^T dt\left[\frac{1}{2}M\dot{\mathbf{R}}_I^2(t)\right]$$
$$= \frac{d}{ds}\int_0^T dt\; M\dot{\mathbf{R}}_I(t)\delta(s-t)$$
$$= \frac{d}{ds}M\dot{\mathbf{R}}_I(s) = M\ddot{\mathbf{R}}_I(s). \quad (18)$$

The second term, instead, demands more attention as it is time non-local. It requires the calculation of

$$\frac{d}{ds}\frac{\delta}{\delta\dot{\mathbf{R}}_I(s)}\int_0^T dt\dot{\mathbf{R}}_I(t)\cdot\int_0^t dt' Q(t-t',\boldsymbol{\zeta})\dot{\mathbf{R}}_I(t'). \quad (19)$$

In order to pass the functional derivative under the integrals of Eq. 19, we expand the domain of the integral over $t'$ to the whole interval $[0,T]$ making use of a Heaviside function. The double integral thus becomes

$$\int_0^T dt\dot{\mathbf{R}}_I(t)\cdot\int_0^T dt'\theta(t-t')Q(t-t',\boldsymbol{\zeta})\dot{\mathbf{R}}_I(t'), \quad (20)$$

whose functional derivative w.r.t. $\dot{\mathbf{R}}_I(s)$ reads

$$\int_0^T dt\;\delta(s-t)\int_0^T dt'\;\theta(t-t')Q(t-t',\boldsymbol{\zeta})\dot{\mathbf{R}}_I(t')$$
$$+\int_0^T dt\;\dot{\mathbf{R}}_I(t)\int_0^T dt'\;\theta(t-t')Q(t-t',\boldsymbol{\zeta})\delta(s-t'). \quad (21)$$

We can now employ the delta functions to get

$$\int_0^T dt'\;\theta(s-t')Q(s-t',\boldsymbol{\zeta})\dot{\mathbf{R}}_I(t') +$$
$$+\int_0^T dt\;\dot{\mathbf{R}}_I(t)\theta(t-s)Q(t-s,\boldsymbol{\zeta}), \quad (22)$$

and then perform a change of variable in the first term of Eq. 22 sending $t'$ in $t$, obtaining

$$\int_0^T dt\;\theta(s-t)Q(s-t,\boldsymbol{\zeta})\dot{\mathbf{R}}_I(t) +$$
$$+\int_0^T dt\;\theta(t-s)Q(t-s,\boldsymbol{\zeta})\dot{\mathbf{R}}_I(t). \quad (23)$$

We can now procede with the differentiation with respect to time $d/ds$ of Eq. 23, which results in

$$\int_0^T dt\;\delta(s-t)Q(s-t,\boldsymbol{\zeta})\dot{\mathbf{R}}_I(t) +$$
$$+\int_0^T dt\;\theta(s-t)\frac{d}{ds}Q(s-t;\boldsymbol{\zeta})\dot{\mathbf{R}}_I(t) +$$
$$-\int_0^T dt\;\delta(t-s)Q(t-s,\boldsymbol{\zeta})\dot{\mathbf{R}}_I(t) +$$
$$+\int_0^T dt\;\theta(t-s)\frac{d}{ds}Q(t-s,\boldsymbol{\zeta})\dot{\mathbf{R}}_I(t), \quad (24)$$

and by exploiting the Dirac deltas and the fact that $\frac{d}{d\tau}Q(\tau,\boldsymbol{\zeta}) = K(\tau,\boldsymbol{\zeta})$ in Eq. 24 one obtains

$$Q(0,\boldsymbol{\zeta})\dot{\mathbf{R}}_I(s) + \int_0^T dt\;\theta(s-t)K(s-t,\boldsymbol{\zeta})\dot{\mathbf{R}}_I(t)$$
$$-Q(0,\boldsymbol{\zeta})\dot{\mathbf{R}}_I(s) - \int_0^T dt\;\theta(t-s)K(t-s,\boldsymbol{\zeta})\dot{\mathbf{R}}_I(t). \quad (25)$$

We can now remove the Heaviside functions inside the integrals by consistently modifying the integration domains, so that Eq. 25 becomes

$$\int_0^s dt\;K(s-t,\boldsymbol{\zeta})\dot{\mathbf{R}}_I(t) - \int_s^T dt\;K(t-s,\boldsymbol{\zeta})\dot{\mathbf{R}}_I(t). \quad (26)$$

We note that the second integral of Eq. 26 depends on times greater than the current time $s$, so that the resulting equation of motion dictates, in contrast to the GLE, that the system dynamics depends not only on the system's past, but also on its future. As pointed out by Ferialdi and Bassi [8], this is a common feature associated to time non-local actions. We stress, however, that it is our aim to exploit such equation of motion as a mean to *generate* the trajectory of the CG particles, in a context where the future evolution of the system is not yet known. Having numerical simulations in mind, we thus *neglect* the second term of Eq. 26 and obtain

$$\frac{d}{ds}\frac{\delta}{\delta\dot{\mathbf{R}}_I(s)}\int_0^T dt\dot{\mathbf{R}}_I(t)\cdot\int_0^t dt' Q(t-t',\boldsymbol{\zeta})\dot{\mathbf{R}}_I(t')$$
$$= \int_0^s dt\;K(s-t)\dot{\mathbf{R}}(t). \quad (27)$$

By combining together Eqs. 16, 18 and 27, one finally recovers the GLE for the CG system presented in Eq. 15. We underline, however, that no *a priori* justification exists for eliminating the future-dependent part of the equation of motion that emerges from the functional derivatives of our effective CG action. It follows that in neglecting such terms an approximation has been performed,

whose degree of accuracy of can only be assessed *a posteriori* once the CG trajectory associated to the GLE is generated, and its statistical properties are compared to the atomistic reference. In this regard, the good agreement we observe between all-atom and CG results, see Fig. 3 and Table I of the main text, suggests that ignoring the future-dependent part is not detrimental; the investigation of whether slight corrections to our time non-local effective CG action in Eq. 13 can be implemented that would render the generalised Euler-Lagrange equations of motion fully compatible with the GLE will be the subject of future work.

## III. DISCRETISATION OF THE ACTION FUNCTIONAL

We now implement a discretisation of Eq. 13 that enables the calculation of $\Sigma[\mathbf{R}, \dot{\mathbf{R}}; \boldsymbol{\zeta}]$ on the discrete CG trajectory $\mathbf{R}(t_n) = \mathbf{R}_n$ obtained by mapping the coordinates of an atomistic molecular dynamics simulation of the system onto their low-resolution counterpart. Such discretisation will be subsequently employed to minimise the action w.r.t. to the properties $\boldsymbol{\zeta}$ that account for the effect of the fast variables, so as to determine the optimised memory kernel $K(t, \boldsymbol{\zeta})$ and the noise $\boldsymbol{\xi}_I(t, \boldsymbol{\zeta})$ appearing in the GLE of the CG particles—see the discussion in Sec. II of the main text.

We treat the noise $\boldsymbol{\xi}_I(t, \boldsymbol{\zeta})$ in Eq. 13 as a 3D coloured noise with unknown autocorrelation $\boldsymbol{L}(t, \boldsymbol{\zeta})$. In the case of discrete times, this can be done by describing it with a moving average process of order $M$ as in [9]. In one dimension such process reads

$$\xi_n = \sum_{j=1}^{M} L_j \eta_{n-j}, \tag{28}$$

where the $\eta_i$ are independent Gaussian random variables with zero mean and unitary variance, while the $L_j$ are functions of the set of properties $\boldsymbol{\zeta}$ contained in the action $\Sigma$. This process can be written for each spatial component $\alpha$ of each particle $I$ in the system as

$$\xi^\alpha_{I,n} = \sum_{j=1}^{M} L^\alpha_j \ \eta^\alpha_{I,n-j}. \tag{29}$$

The action $\Sigma[\mathbf{R}, \dot{\mathbf{R}}; \boldsymbol{\zeta}]$ in Eq. 13 can be discretised as follows:

$$\Sigma[\mathbf{R}, \dot{\mathbf{R}}, \boldsymbol{\zeta}] \simeq \Delta t \sum_{I=1}^{N_B} \sum_{n=M}^{N} \Bigg[ K_R(\dot{\mathbf{R}}_{I,n}) + \\ - \sum_J \frac{1}{2} U_2(\mathbf{R}_{I,n}, \mathbf{R}_{J,n}) + \Delta t \left( \dot{\mathbf{R}}_{I,n} \cdot \sum_{i=n-M}^{n} Q_{n-i} \dot{\mathbf{R}}_{I,i} \right) \\ + \mathbf{R}_{I,n} \cdot \boldsymbol{\xi}_{I,n} \Bigg]. \tag{30}$$

In Eq. 30, $\Delta t$ and $N$ are respectively the time step and the total number of snapshots of the all-atom simulation, while $N_B$ is the number of CG particles in the system; we have approximated the many-body potential of mean force acting among the CG sites as a sum of pair interactions $U_2(\mathbf{R}_I, \mathbf{R}_J)$, see Sec. IV A of the main text. The sum over $J$ in Eq. 30 thus runs over the (instantaneous) neighbors of the $I^{th}$ bead that contribute to its potential energy. Furthermore, $Q_{i-j}$ represents the discretised form of $Q(t - t', \boldsymbol{\zeta})$, where for the sake of notational simplicity we have omitted in the right-hand side of Eq. 30—and will omit in the following—the dependence of $Q$ and of the noise $\boldsymbol{\xi}_I$ on the properties $\boldsymbol{\zeta}$. Finally, the index $M$ is the number of time steps prior to the current one $n$ on which the memory kernel acts, that is, in analogy with Eq. 29 we assume $Q_{i-j} = 0$ for $i - j > M$, so that the memory has a finite extension in time.

The action in Eq. 30 can be now decomposed as

$$\Sigma = \Sigma_K[\dot{\mathbf{R}}] + \Sigma_U[\mathbf{R}] + \sum_{\alpha=x,y,z} \bar{\Sigma}^\alpha[R^\alpha, \dot{R}^\alpha, \boldsymbol{\zeta}]. \tag{31}$$

Critically, the kinetic and potential factors $\Sigma_K$ and $\Sigma_U$ in Eq. 31 do not depend on the parameters $\boldsymbol{\zeta}$ entering in $\boldsymbol{\xi}_{I,n}$ and $Q_n$, over which the action, once computed over the CG trajectory, will be subsequently minimised: as such, these terms will be neglected in the following. On the other hand $\bar{\Sigma}^\alpha$, with $\alpha \in \{x, y, z\}$, reads

$$\bar{\Sigma}^\alpha[R^\alpha, \dot{R}^\alpha, \boldsymbol{\zeta}^\alpha] = \sum_{I=1}^{N_B} \left\{ \Delta t \sum_{n=M}^{N} \left[ \Delta t \ \dot{R}^\alpha_{I,n} \sum_{i=n-M}^{n} Q^\alpha_{n-i} \dot{R}^\alpha_{I,i} + R^\alpha_{I,n} \sum_{j=1}^{M} L^\alpha_j \ \eta^\alpha_{I,n-j} \right] \right\}. \tag{32}$$

We note that in contrast to Eq. 30 and 31, in which $Q_i \delta^{\alpha\beta} = Q_i^{\alpha\beta}$ was implicitly by all means an isotropic tensor, in Eq. 32 we now allowed each spatial component $\alpha$ to be in principle related to a *different* $Q^\alpha(\tau)$, with $\frac{d}{d\tau} Q^\alpha(\tau) = K^\alpha(\tau)$. Together with its dependence on the set of $L^\alpha_j$, we now treat each $\bar{\Sigma}^\alpha[R^\alpha, \dot{R}^\alpha, \boldsymbol{\zeta}^\alpha]$ *as a function of its own set of properties* $\boldsymbol{\zeta}^\alpha$, so that the minimisation of the global action in Eq. 31 can be obtained by the separate minimisation of each $\bar{\Sigma}^\alpha$ w.r.t. to the corresponding $\boldsymbol{\zeta}^\alpha$. Rotational invariance of the all-atom—and conse-

quently of the CG—system, on the other hand, requires $Q_i^x = Q_i^y = Q_i^z$, or equivalently $K_i^x = K_i^y = K_i^z$: this can be verified *a posteriori* once the independent minimisations over the spatial directions are performed, and the three set of optimal parameters $\boldsymbol{\zeta}^x, \boldsymbol{\zeta}^y, \boldsymbol{\zeta}^z$ are employed in the calculation of the associated memory kernels. We will come back to this discussion in Sec. IV.

Let us now consider all the factors entering $\bar{\Sigma}^\alpha[R^\alpha, \dot{R}^\alpha, \boldsymbol{\zeta}^\alpha]$ in Eq. 32. We begin with the noise term, which in extended form reads

$$\sum_{I=1}^{N_B} \Delta t \sum_{n=M}^{N} R_{I,n}^\alpha \begin{bmatrix} \eta_{I,n-1}^\alpha \\ \eta_{I,n-2}^\alpha \\ \cdots \\ \eta_{I,n-M}^\alpha \end{bmatrix}^T \cdot \begin{bmatrix} L_1^\alpha \\ L_2^\alpha \\ \vdots \\ L_M^\alpha \end{bmatrix}.$$

This can be written in a more compact notation as

$$\Delta t \underbrace{\begin{bmatrix} \sum_{I=1}^{N_B} \sum_{n=M}^{N} \eta_{I,n-1}^\alpha \; R_{I,n}^\alpha \\ \sum_{I=1}^{N_B} \sum_{n=M}^{N} \eta_{I,n-2}^\alpha \; R_{I,n}^\alpha \\ \cdots \\ \sum_{I=1}^{N_B} \sum_{n=M}^{N} \eta_{n-M}^\alpha \; R_{I,n}^\alpha \end{bmatrix}^T}_{\boldsymbol{\Xi}^\alpha} \cdot \boldsymbol{L}^\alpha, \tag{33}$$

and, via the definition of the vector $\boldsymbol{\Xi}^\alpha$, as

$$\Delta t \left[\Xi_1^\alpha, \cdots, \Xi_M^\alpha\right] \cdot \boldsymbol{L}^\alpha. \tag{34}$$

An analogous analysis of the memory term in Eq. 32 requires more attention and longer calculations. In vector notation, this reads

$$\Delta t^2 \sum_{I=1}^{N_B} \sum_{n=M}^{N} \dot{R}_{I,n}^\alpha \left[\dot{R}_{I,n}^\alpha, \dot{R}_{I,n-1}^\alpha, \cdots, \dot{R}_{I,n-M}^\alpha\right] \cdot \begin{bmatrix} Q_0^\alpha \\ Q_1^\alpha \\ \vdots \\ Q_M^\alpha \end{bmatrix}.$$

Also in this case a more compact form can be employed, namely

$$\Delta t^2 \underbrace{\begin{bmatrix} \sum_{I=1}^{N_B} \sum_{n=M}^{N} \dot{R}_{I,n}^\alpha \dot{R}_{I,n}^\alpha \\ \sum_{I=1}^{N_B} \sum_{n=M}^{N} \dot{R}_{I,n}^\alpha \dot{R}_{I,n-1}^\alpha \\ \cdots \\ \sum_{I=1}^{N_B} \sum_{n=M}^{N} \dot{R}_{I,n}^\alpha \dot{R}_{I,n-M}^\alpha \end{bmatrix}^T}_{\boldsymbol{\Gamma}^\alpha} \cdot \boldsymbol{Q}^\alpha,$$

or, equivalently,

$$\Delta t^2 \left[\Gamma_0^\alpha, \Gamma_1^\alpha, \cdots, \Gamma_M^\alpha\right] \cdot \boldsymbol{Q}^\alpha, \tag{35}$$

where we identified the first factor with the vector $\boldsymbol{\Gamma}^\alpha$.

Given these definitions, the discretised action in Eq. 32 can be written in the following simpler form:

$$\bar{\Sigma}^\alpha[R^\alpha, \dot{R}^\alpha, \boldsymbol{\zeta}^\alpha] = \Delta t^2 \; \boldsymbol{\Gamma}^{\boldsymbol{\alpha}} \cdot \boldsymbol{Q}^\alpha + \Delta t \; \boldsymbol{\Xi}^\alpha \cdot \boldsymbol{L}^\alpha. \tag{36}$$

At the same time, we are interested in the memory kernel $K^\alpha(t)$, and not in its primitive $Q^\alpha(t)$. We thus have to rewrite the scalar product in Eq. 35 by performing a further approximation. We know from the initial assumptions that

$$\frac{d}{dt} Q^\alpha(t) = K^\alpha(t), \tag{37}$$

and we can rely on the forward finite difference approximation for computing the time-discretised derivatives, which provides

$$\begin{aligned} K_0^\alpha &= \frac{Q_1^\alpha - Q_0^\alpha}{\Delta t}, \\ K_1^\alpha &= \frac{Q_2^\alpha - Q_1^\alpha}{\Delta t}, \\ &\vdots \\ K_{M-1}^\alpha &= \frac{Q_M^\alpha - Q_{M-1}^\alpha}{\Delta t}. \end{aligned}$$

Such relations can be inverted to obtain

$$Q_k^\alpha = \Delta t \sum_{j=0}^{k-1} K_j^\alpha, \tag{38}$$

via the Euler method, where we assume that $Q_0^\alpha = 0$. Eq. 38 can now be plugged into Eq. 35, resulting in

$$\begin{aligned} &\Gamma_0^\alpha \cancelto{0}{Q_0^\alpha} + \Gamma_1^\alpha Q_1^\alpha + \cdots + \Gamma_M^\alpha Q_M^\alpha = \\ &\Delta t (\Gamma_1^\alpha K_0^\alpha + \Gamma_2^\alpha (K_0^\alpha + K_1^\alpha) + \cdots + \\ &\cdots + \Gamma_M^\alpha (K_0^\alpha + K_1^\alpha + \cdots + K_{M-1}^\alpha)). \end{aligned}$$

We note that this expression can be rearranged grouping the $K_i^\alpha$ values, that is,

$$\begin{aligned} &\Delta t [K_0^\alpha (\Gamma_1^\alpha + \Gamma_2^\alpha + \cdots + \Gamma_M^\alpha) + \\ &K_1^\alpha (\Gamma_2^\alpha + \Gamma_3^\alpha + \cdots + \Gamma_M^\alpha) + \\ &\cdots + K_{M-1}^\alpha \Gamma_M^\alpha], \end{aligned}$$

or, in vector form,

$$\Delta t \left[\tilde{\Gamma}_1^\alpha, \tilde{\Gamma}_2^\alpha, \cdots, \tilde{\Gamma}_M^\alpha\right] \cdot \boldsymbol{K}^\alpha, \tag{39}$$

with $\tilde{\Gamma}_k^\alpha = \sum_{j=k}^{M} \Gamma_j^\alpha$ and $\boldsymbol{K}^\alpha = [K_0^\alpha, K_1^\alpha, ..., K_{M-1}^\alpha]$.

Finally, in order to perform the minimisation we need to introduce some constraints on the memory kernel $K^\alpha$ in order to stabilise the numerical solution of the problem, including one concerning its integral, see Sec. IV and V. These constraints are accounted for in the function to be minimised using the Lagrangian multiplier formalism, which in a general fashion reads

$$\boldsymbol{\mu}^\alpha \cdot \tilde{\boldsymbol{C}}^\alpha, \tag{40}$$

with $\boldsymbol{\mu}^\alpha$ being a vector of Lagrangian multipliers and $\tilde{\boldsymbol{C}}^\alpha$ a set of constraints that are functionals of the kernel.

By combining Eqs. 34, 39 and 40, we can finally write the complete expression of the discrete action $\bar{\Sigma}^\alpha$ along each spatial component in compact form:

$$\boxed{\bar{\Sigma}^\alpha = \Delta t^3 \; \tilde{\boldsymbol{\Gamma}}^{\boldsymbol{\alpha}} \cdot \boldsymbol{K}^\alpha + \Delta t \; \boldsymbol{\Xi}^\alpha \cdot \boldsymbol{L}^\alpha - \boldsymbol{\mu}^\alpha \cdot \tilde{\boldsymbol{C}}^\alpha} \tag{41}$$

For the subsequent analysis, given the CG trajectory $\mathbf{R}_n$ each of the actions $\bar{\Sigma}^\alpha$ can be formally seen as a stochastic variable, as it embodies a set of Gaussian i.i.d. random variables $\boldsymbol{\eta}^\alpha$. Moreover, it is also dependent on a set of yet unknown parameters $\boldsymbol{\zeta}^\alpha$ representing the effect of the fast variables, with respect to which the minimisation will be carried out. Hence, $\bar{\Sigma}^\alpha \doteq \bar{\Sigma}^\alpha(\boldsymbol{\zeta}^\alpha, \boldsymbol{\eta}^\alpha)$.

The crucial point now consists in finding an appropriate parametrisation of the functions $K^\alpha(t)$ and of the noise factors $L_j^\alpha$, and then searching for the values of $\boldsymbol{\zeta}^\alpha$ that minimise the actions $\bar{\Sigma}^\alpha$.

## IV. PARAMETER ESTIMATION AND OPTIMIZATION

Once the discretised version of the action has been obtained, see Eq. 41, we need to minimize it with respect to the properties $\boldsymbol{\zeta}^\alpha$ on which the kernel $K_i^\alpha$ and coefficients $L_i^\alpha$ appearing in the noise formally depend. Therefore the problem, for each spatial component $\alpha \in \{x, y, z\}$, reads

$$\begin{aligned}
&\min_{\boldsymbol{\zeta}^\alpha, \boldsymbol{\mu}^\alpha} \bar{\Sigma}^\alpha(\boldsymbol{\zeta}^\alpha, \boldsymbol{\eta}^\alpha) = \\
&\min_{\boldsymbol{\zeta}^\alpha, \boldsymbol{\mu}^\alpha} \Big( \Delta t^3 \, \tilde{\boldsymbol{\Gamma}}^{\boldsymbol{\alpha}} \cdot \boldsymbol{K}^\alpha(\boldsymbol{\zeta}^\alpha) + \\
&+ \Delta t \; \boldsymbol{\Xi}^\alpha \cdot \boldsymbol{L}^\alpha(\boldsymbol{\zeta}^\alpha) - \boldsymbol{\mu}^\alpha \cdot \tilde{\boldsymbol{C}}^\alpha(\boldsymbol{\zeta}^\alpha) \Big) , \qquad (42)
\end{aligned}$$

where the properties $\boldsymbol{\zeta}^\alpha$ enter the constraints $\tilde{\boldsymbol{C}}^\alpha$ via the kernel, see Sec. V, and we also perform the formal minimization with respect to $\boldsymbol{\mu}^\alpha$ necessary to implement the constraints.

The general idea to actually perform the optimization is to choose a functional form for $K^\alpha(t, \boldsymbol{\zeta}^\alpha)$ dependent on a set of properties $\boldsymbol{\zeta}^\alpha$, and then find the values of these parameters that minimise each action $\bar{\Sigma}^\alpha(\boldsymbol{\zeta}^\alpha, \boldsymbol{\eta}^\alpha)$.

Before approaching this task, however, let us first focus our attention on the noise term in Eq. 42, $\Delta t \; \boldsymbol{\Xi}^\alpha \cdot \boldsymbol{L}^\alpha$. From stochastic optimisation theory [10], we know that the minimum of a function $g(x, \eta)$ dependent on some stochastic value $\eta$ is the minimum of the average,

$$\min_x g(x, \eta) = \min_x \mathbb{E}[g(x, \eta)],$$

where $\mathbb{E}[\cdot]$ is the expectation value of an observable. Hence, we write our minimization problem as

$$\min_{\boldsymbol{\zeta}^\alpha, \boldsymbol{\mu}^\alpha} \bar{\Sigma}^\alpha(\boldsymbol{\zeta}^\alpha, \boldsymbol{\eta}^\alpha) = \min_{\boldsymbol{\zeta}^\alpha, \boldsymbol{\mu}^\alpha} \mathbb{E}\left[\bar{\Sigma}^\alpha(\boldsymbol{\zeta}^\alpha, \boldsymbol{\eta}^\alpha)\right] = \qquad (43)$$

$$\min_{\boldsymbol{\zeta}^\alpha, \boldsymbol{\mu}^\alpha} \mathbb{E}\left[\Delta t^3 \, \tilde{\boldsymbol{\Gamma}}^{\boldsymbol{\alpha}} \cdot \boldsymbol{K}^\alpha + \Delta t \; \boldsymbol{\Xi}^\alpha \cdot \boldsymbol{L}^\alpha - \boldsymbol{\mu}^\alpha \cdot \tilde{\boldsymbol{C}}^\alpha\right] . \qquad (44)$$

Now, using the linearity of the expectation $\mathbb{E}[\cdot]$ and the fact that the expectation of a constant is the constant itself, the expression becomes

$$\min_{\boldsymbol{\zeta}^\alpha, \boldsymbol{\mu}^\alpha} \left(\Delta t^3 \, \tilde{\boldsymbol{\Gamma}}^{\boldsymbol{\alpha}} \cdot \boldsymbol{K}^\alpha + \Delta t \; \mathbb{E}\left[\boldsymbol{\Xi}^\alpha\right] \cdot \boldsymbol{L}^\alpha - \boldsymbol{\mu}^\alpha \cdot \tilde{\boldsymbol{C}}^\alpha\right) . \qquad (45)$$

Moreover, again for the linearity of $\mathbb{E}[\cdot]$, one has

$$\begin{aligned}
\mathbb{E}[\boldsymbol{\Xi}_z^\alpha] &= \mathbb{E}\left[\sum_{I=1}^{N_B} \sum_{n=M}^{N} \eta_{n-z}^\alpha \; R_{I,n}^\alpha\right] = \\
&= \sum_{I=1}^{N_B} \sum_{n=M}^{N} \mathbb{E}\left[\eta_{n-z}^\alpha\right] \; R_{I,n}^\alpha = 0, \qquad (46)
\end{aligned}$$

since the Gaussian random variables $\eta_j^\alpha$ have expectation zero $\mathbb{E}[\eta_j^\alpha] = 0$. Here $z \in [1, .., M]$ identifies every component of $\boldsymbol{\Xi}^\alpha$.

The formal minimisation problem can thus be recast in the following form:

$$\min_{\boldsymbol{\zeta}^\alpha, \boldsymbol{\mu}^\alpha} \bar{\Sigma}^\alpha(\boldsymbol{\zeta}^\alpha, \boldsymbol{\eta}^\alpha) = \min_{\boldsymbol{\zeta}^\alpha, \boldsymbol{\mu}^\alpha} \left(\Delta t^3 \, \tilde{\boldsymbol{\Gamma}}^{\boldsymbol{\alpha}} \cdot \boldsymbol{K}^\alpha - \boldsymbol{\mu}^\alpha \cdot \tilde{\boldsymbol{C}}^\alpha\right) , \qquad (47)$$

where, importantly, the parameters $\boldsymbol{L}^\alpha$ no longer come into play and can instead be obtained *a posteriori* once the kernel is known, see Sec. IV B.[2]

In order to minimise Eq. 47, we now define each kernel $K^\alpha(t) = f(t, \boldsymbol{\zeta}^\alpha)$ to be a smooth function of $t$ that depends on the set of parameters $\boldsymbol{\zeta}^\alpha$. We evaluate it in $t = n\Delta t$ for $n \in [0, M-1]$, so that

$$\boldsymbol{K}^\alpha = \begin{bmatrix} K_0^\alpha \\ K_1^\alpha \\ \vdots \\ K_{M-1}^\alpha \end{bmatrix} = \begin{bmatrix} f(0, \boldsymbol{\zeta}^\alpha) \\ f(\Delta t, \boldsymbol{\zeta}^\alpha) \\ \vdots \\ f((M-1)\Delta t, \boldsymbol{\zeta}^\alpha) \end{bmatrix} , \qquad (48)$$

and by plugging this vector into Eq. 47 we obtain

$$\begin{aligned}
&\min_{\boldsymbol{\zeta}^\alpha, \boldsymbol{\mu}^\alpha} \bar{\Sigma}^\alpha(\boldsymbol{\zeta}^\alpha, \boldsymbol{\eta}^\alpha) = \\
&\min_{\boldsymbol{\zeta}^\alpha, \boldsymbol{\mu}^\alpha} \left(\Delta t^3 \sum_{i=1}^{M} \tilde{\Gamma}_i^\alpha f((i-1)\Delta t, \boldsymbol{\zeta}^\alpha) - \boldsymbol{\mu}^\alpha \cdot \tilde{\boldsymbol{C}}^\alpha\right) . \qquad (49)
\end{aligned}$$

[2] We recall that the stochastic terms $\boldsymbol{\xi}_J(t, \boldsymbol{\zeta})$ were here introduced as a proxy for the deterministic forces $\boldsymbol{\mathcal{F}}_J(t, \boldsymbol{\zeta})$ that act on the slow, CG variables as a consequence of the MZ projection, see Eqs. 12, 13 and the comment in Fn. 1. Having obtained that the $\boldsymbol{\xi}_J(t, \boldsymbol{\zeta})$ do not affect the minimisation problem, it is interesting to briefly comment what would happen if the original $\boldsymbol{\mathcal{F}}_J(t, \boldsymbol{\zeta})$ were employed in the definition of the effective CG action. As evidenced by Eq. 13, such forces would enter a now fully deterministic $\Sigma[\mathbf{R}, \dot{\mathbf{R}}; \boldsymbol{\zeta}]$ through factors $F_J(\boldsymbol{\zeta}) = \int_0^T dt \; \boldsymbol{\mathcal{F}}_J(t, \boldsymbol{\zeta}) \cdot \mathbf{R}_J(t)$, which should in principle be accounted for in the minimisation as they depend on the fast dynamics parameters $\boldsymbol{\zeta}$. At the same time, provided that the forces $\boldsymbol{\mathcal{F}}_J$ fluctuate very rapidly in $t$ compared to the $\mathbf{R}_J$—as it is commonly assumed in the literature [6]—each integral $F_J$ can be effectively considered to couple a slowly varying CG coordinate to a time average, performed over short timescales, of the associated deterministic force. For systems in equilibrium it is reasonable to expect such time averages to vanish, so that the ensemble of $F_J$ becomes independent on $\boldsymbol{\zeta}$ and can be neglected in the minimisation problem, with the deterministic framework thus becoming equal to its stochastic counterpart. It follows that, under the aforementioned assumption of time scales decoupling, one can consider our whole optimisation workflow as if it was done in presence of the real, MZ deterministic forces $\boldsymbol{\mathcal{F}}_J$, where only in the end, after the kernel is determined, these are identified with stochastic variables $\boldsymbol{\xi}_J$.

In conclusion, the minimisation problem for each spatial dimension can be stated in a more familiar form, namely

$$\boxed{\begin{array}{c}\min_{\boldsymbol{\zeta}^\alpha}\ \Delta t^3 \sum_{i=1}^{M} \tilde{\Gamma}_i^\alpha f((i-1)\Delta t, \boldsymbol{\zeta}^\alpha) \\ \text{subj. to}\ \ \tilde{\boldsymbol{C}}^\alpha = 0.\end{array}} \tag{50}$$

### A. Minimisation of the discretised action

As previously discussed, the minimisation of the discrete action in Eq. 50 is attained through the introduction of three independent memory kernels $K^\alpha(t, \boldsymbol{\zeta}^\alpha)$, $\alpha \in \{x, y, z\}$, where each kernel depends on a set parameter $\boldsymbol{\zeta}^\alpha$ over which the optimisation is performed. In this work, the memory kernel associated to each spatial direction was assumed to be positive and defined by the following functional form:

$$K(t, \boldsymbol{\zeta}) = K(t, a, \boldsymbol{b}) = g(t, a) b(t, \boldsymbol{b}) = e^{-at^2} b(t, \boldsymbol{b}), \tag{51}$$

where for the sake of notational simplicity we have omitted—and will omit in the following—the Cartesian indices in both the kernel and the associated parameters. Eq. 51 consists of a global Gaussian prefactor $g(t, a)$ modulated by a term $b(t, \boldsymbol{b})$, the latter being is a positive function of time such that $b(t_k) = b_k$ at time $t_k = k\Delta t$. In this way, the kernel—actually, the independent kernel associated to each spatial direction—can be treated as a function of the parameter $a$ and of the vector of parameters $\boldsymbol{b} = [b_0, b_2, ..., b_{M-1}]$ that represent the properties $\boldsymbol{\zeta}$ and have to be varied so as to achieve the minimisation of the discrete action in Eq. 50. The kernel $K$ can thus be explicitly written as

$$K(t, a, \boldsymbol{b}) = e^{-at^2} b(t), \tag{52}$$

or, equivalently, as

$$K(t_k, a, \boldsymbol{b}) = e^{-at_k^2} b_k. \tag{53}$$

Importantly, we note that our prescription of fixing a global, Gaussian prefactor in the kernel differs from the usual choice of parametrising it as a series of exponentials or damped oscillators [6, 11–14]. At the same time this is not a limiting constraint, as the vector $\boldsymbol{b}$ can—and actually does, *vide infra*—generate a significant modulation of the Gaussian term $g(t, a)$ as a consequence of the minimisation procedure. Given our choice of the functional form of $K$, the optimisation problem of Eq. 50 in its discretised form and for each spatial direction becomes

$$\min_{\mathbf{a},\mathbf{b}}\ \Delta t^3 \sum_{k=1}^{M} \tilde{\Gamma}_k\ e^{-at_{k-1}^2} b_{k-1}, \tag{54}$$

where the additional constraints $\tilde{\boldsymbol{C}}^\alpha$ appearing in Eq. 50 have now been intentionally disregarded, the necessity of their introduction being addressed in the following.

The minimisation of Eq. 54 with the aim of determining the optimal kernel $K$ is rendered nonlinear by the presence of the parameter $a$. Rather than tackling the complete problem, to identify its solution we resorted to a two-step approach (see numerical details below), first determining the "optimal" value of $a$, $\tilde{a}$, and subsequently optimising the vector $\boldsymbol{b}$ keeping $\tilde{a}$ fixed. As a consequence of our *Ansatz* for the kernel, however, we note that once the parameter $\tilde{a}$ is given Eq. 54 simply amounts at the minimisation of a hyperplane in the set of coefficients $b_k$, $k = 0, ..., M-1$, a procedure that, in absence of additional conditions, would result in unbounded solutions. It is at this stage that the introduction of two constraints on the kernel $K$ proves necessary to regularise the optimisation workflow. Specifically, the first constraint $\tilde{C}_1$ concerns the integral of $K$, whose relation to the diffusion coefficient $D$ [15], see Sec.V, is enforced by requiring

$$0 \equiv \tilde{C}_1 = \int_0^{\bar{t}_M} dt\ K(t, \tilde{a}, \boldsymbol{b}) - \frac{k_B T}{D}, \tag{55}$$

where $\tilde{a}$ is fixed to the optimised value and the integration has been truncated at $\bar{t}_M = M\Delta t$ because of the decay of the kernel. *Via* this condition, the kernel that minimises Eq. 54 is thus sought in the space of all possible functions that reproduce the diffusion coefficient of the system. Moreover, the integral in Eq. 55 can be interpreted as the $L^2$ inner product $\langle g, b\rangle$ between the the two functions defining the kernel. As we assume $K(t) \geq 0$, by combining the constraint in Eq. 55 with the Cauchy-Schwarz inequality in the case of positive functions, $0 \leq \langle g, b\rangle \leq ||g||_{L^2}||b||_{L^2}$ where $||\cdot||_{L^2}$ is the $L^2$ norm induced by the scalar product, we can also derive another auxiliary condition on $b(t)$ that is included as an additional requirement. The optimisation problem of Eq. 54, given the value of $\tilde{a}$ and explicitly accounting for the introduced constraints, can hence be recast in

$$\min_{\boldsymbol{b}}\ \Delta t^3 \sum_{k=1}^{M} \tilde{\Gamma}_k\ e^{-\tilde{a}t_{k-1}^2} b_{k-1}, \tag{56}$$

$$\text{subj. to}: \sum_{k=0}^{M-1} e^{-\tilde{a}t_k^2} b_k \Delta t = \frac{k_B T}{D}, \tag{57}$$

$$||b||_{L^2} = \left(\sum_{k=0}^{M-1} b_k^2 \Delta t\right)^{\frac{1}{2}} \geq \frac{k_B T}{D||g||_{L^2}}, \tag{58}$$

where, analogously to $||b||_{L^2}$, $||g||_{L^2}$ is the discretised $L^2$ norm of the optimised Gaussian factor $g(t, \tilde{a})$ defined in Eq. 51. We note that the condition in Eq. 58 is a direct consequence of the Cauchy-Schwarz inequality, and is thus satisfied for any $b(t) \geq 0$ compatible with the constraint of Eq. 57. Nonetheless, as we will discuss in the following, the existence of a lower bound for $||b||_{L^2}$ proves beneficial to the convergence of the optimisation protocol. More generally, it is important to stress that the necessity for the introduction of both the constraints in Eq. 57 and Eq. 58 arises as a direct consequence of our

choice for the *Ansatz* of the kernel, see Eq. 52, and of the overall approach we employed for the optimisation. We cannot exclude that in the case of a fully nonlinear function $K(t, \boldsymbol{\zeta})$ of the parameters $\boldsymbol{\zeta}$ the action minimisation could be safely performed also in absence of additional conditions. For example, it would be interesting to represent the kernel as a parametric series of exponentials or damped oscillators as in Refs. [6, 11–14], a choice which, in contrast to the linear case, would render the minimisation problem bounded. Critically, by employing such a parametrisation for $K$ one could further resort to an extended Markovian process to integrate the CG equations of motion, resulting in higher computational efficiency with respect to the non-Markovian case. Work in this direction is in progress.

Moving to the technical details associated to the numerical implementation, in the calculation of the discretised action for the water system we chose the number of time steps on which the memory kernel $K$ acts to be $M = 500$—that is, $K(t, a, \boldsymbol{b}) = 0$ for $t \geq \bar{t}_M = 1$ ps—and took into account $N = 3 \times 10^4$ time steps of the reference all-atom simulation. As previously discussed, the minimisation in Eq. 54 was then performed in two stages, where we separately optimised the parameter $a$ and the vector $\boldsymbol{b}$; more specifically, we initially set the modulation term $b(t, \boldsymbol{b}) = 1$ in Eq. 51, thus considering a preliminary, purely Gaussian kernel $K(t, a) = g(t, a)$. The "optimal" value of $a$, $\tilde{a}$, was then determined by requiring that the integral of $g(t, \tilde{a})$ is related to the all-atom diffusion coefficient via Eq. 55. The kernel generated by this analysis is presented in the inset of Fig. 1.

Given $\tilde{a}$, we subsequently moved to the second stage of the procedure, namely the numerical optimisation of the modulation vector $\boldsymbol{b}$. To this end, we kept $a$ fixed to $\tilde{a}$ and determined the optimal value $\tilde{\boldsymbol{b}}$ through a minimisation, with respect to $\boldsymbol{b}$ alone, of Eq. 56 subject to the constraints defined in Eqs. 57 and 58.

A few remarks about this second stage are in order, especially as far as Eq. 58 is concerned. Indeed, in absence of any condition on the sign of the vector $\boldsymbol{b}$ and its norm $||b||_{L^2}$, the numerical optimisation workflow displayed the tendency of generating unstable solutions in the form of vectors comprising some negative components. The magnitude of such components increased with the optimisation step, consequently resulting in a growth of the norm $||b||_{L^2}$ while keeping the constraint of Eq. 57 satisfied. A growth in the magnitude of the components of the vector $\boldsymbol{b}$ is not surprising, and can arise as a consequence of the unboundedness of the cost function to be minimised, see Eq. 56, even if the constraint on the integral of the kernel is enforced. More critically, the dynamics generated by the GLE embodying these negative kernels was found to not reproduce the correct velocity correlation function of the water system. To tackle the problem, we thus restricted the choice of the possible $\boldsymbol{b}$ to vectors with positive components only, and further required the modulation of the kernel induced by $\boldsymbol{b}$ to be globally *as small as possible*, that is, we asked for the associated

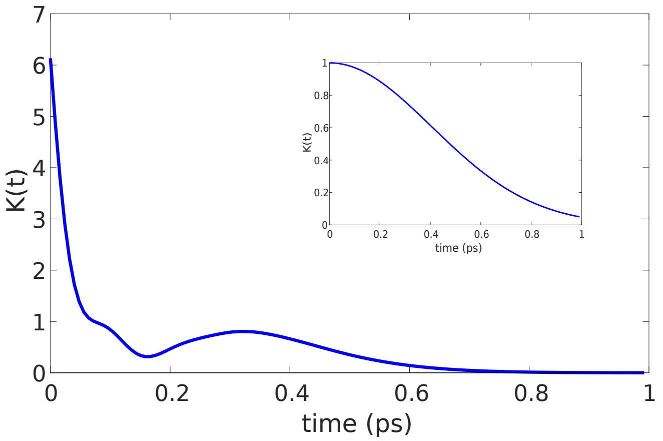


**FIG. 1:** *Main panel*: Optimised memory kernel $K(t, \tilde{a}, \tilde{\boldsymbol{b}})$, see Eq. 51, obtained through a minimisation of the discretised time-non-local effective CG action. This kernel, combined with the associated optimised noise parameters $\boldsymbol{\xi}$ and the CG potential $U$, was employed in the numerical integration of the GLE for the CG water system and provided the results displayed in Fig. 3 and Table I of the main text. *Inset*: Gaussian kernel $K(t, \tilde{a}) = g(t, \tilde{a}) = \exp[-\tilde{a}t^2]$, see Eq. 51, obtained at the first stage of the optimisation workflow. The parameter $\tilde{a}$ was determined by imposing the relation between the integral of $g(t, \tilde{a})$ and the diffusion coefficient reported in Eq. 55.

norm $||b||_{L^2}$ to be close to the lower bound reported in Eq 58.

Overall, we proceeded as follows: we first minimised Eq. 56 subject to Eq. 57 by treating the constraint in Eq. 58 as an equality, and stored the obtained kernel $K^{(0)} = K(t, \tilde{a}, \tilde{\boldsymbol{b}}^{(0)})$, where $\tilde{\boldsymbol{b}}^{(0)}$ is the optimal vector of parameters determined according to these prescriptions. We note that enforcing an equality in Eq. 58 in principle amounts at requiring $\tilde{b}^{(0)}(t)$ to be a multiple of $g(t, \tilde{a})$; because of the intrinsic approximate nature of the numeric approach, however, such a parallelism was not observed, and deviations between $\tilde{b}^{(0)}(t)$ and $g(t, \tilde{a})$ arose already at this preliminary step. We then kept on considering Eq. 58 as an equality but increased its right-hand side by a small amount $\epsilon$, i.e., setting it to $k_B T / D ||g||_{L^2} + \epsilon$, solved again the problem for the new optimal vector $\tilde{\boldsymbol{b}}^{(1)}$, and stored the resulting kernel $K^{(1)}$. We continued this procedure by increasing sequentially the known term by $\epsilon$ and solving and storing the results, stopping the iterations when the minimum of the kernel that was produced by the optimization was less or equal to zero. Finally, we took as overall optimal kernel the average of the kernels $K^{(z)}$ obtained at the various steps. We can summarise the workflow in the following pseudo-code:

*set* $q = 0$

**while** $\min_k K^{(q)}(t_k) > 0$ **do**

*solve*

$$\min_{\boldsymbol{b}} \ \Delta t^3 \sum_{k=1}^{M} \tilde{\Gamma}_k \ e^{-\tilde{a} t_{k-1}^2} b_{k-1},$$

$$\text{subj. to}: \sum_{k=0}^{M-1} e^{-\tilde{a}t_k^2} b_k \Delta t = \frac{k_B T}{D},$$
$$\left(\sum_{k=0}^{M-1} b_k^2 \Delta t\right)^{\frac{1}{2}} = \frac{k_B T}{D||g||_{L^2}} + q\epsilon,$$

*store* $K^{(q)}(t_k),\ k = 0, .., M-1$
$q \leftarrow q + 1$
**end while**
$K^{opt}(t_k) = \frac{1}{q} \sum_{z=0}^{q-1} K^{(z)}(t_k),\ k = 0, .., M-1.$

where $K^{(z)}(t_k)$ is the short form for the discrete kernel $K(t_k, \tilde{a}, \tilde{\boldsymbol{b}}^{(z)})$ obtained at the $z$-th iteration of the process. The initial guess for $\boldsymbol{b}$ for all procedure's steps was $b_k = 1\ \forall k$, namely the same prescription employed in the first stage of the overall parameter optimisation workflow. As for $\epsilon$, its value has to be small enough to provide a series of memory kernels whose minimum approaches zero smoothly, thus avoiding sudden sub-zero jumps of the solution. After a systematic scan of the results associated to different choices of $\epsilon$ we set it to $0.04\ \frac{kg^{1/2}}{mol^{1/2}} \frac{1}{ps}$, and 8 optimisation steps were performed before the minimum of the kernel reached negative values.

All minimisations of the discrete action were achieved by relying on a Nelder-Mead simplex algorithm that explicitly accounted for the presence of the constraints [16]. Furthermore, we stress that, although in the preceding discussion we have omitted the dependence of the kernel on the Cartesian index, the minimisation was actually performed independently along the three coordinate axes, see Eq. 50, so that the procedure provided us with three optimised kernel $K^x(t)$, $K^y(t)$ and $K^z(t)$. Such kernels, however, turned out to be identical, so that, as expected, rotational invariance was found to be preserved in the GLE dictating the dynamics of the CG system.

The optimised memory kernel $K(t)$ obtained at the end of the workflow is presented in the main panel of Fig. 1. We note that the action minimisation procedure generates a significant modulation of the preliminary, purely Gaussian kernel $g(t, \tilde{a})$, see Eqs. 52 and 53; more precisely, the optimal $K(t)$ displays a higher and steeper peak in the vicinity of $t = 0$ compared to its Gaussian counterpart, as well as a faster decaying behavior. In addition to these overall, global properties, we further observe the emergence of nontrivial local features in the final kernel, namely the presence of oscillations that occur at intermediate timescales.

Finally, it is important to quantify the sensitivity of our results with to the length of the atomistic simulation employed in the parametrisation of the kernel $K(t)$. For this purpose, we divided the full trajectory in two equal chunks of $N = 1.5 \times 10^4$ time steps each and performed two independent optimisations by relying on the previously described protocol. A comparison of the two kernels we obtain, together with the one associated to the full trajectory, is presented in Fig. 2, and highlights that the three curves are indistinguishable on the scale of the figure, thus confirming the stability of our results.

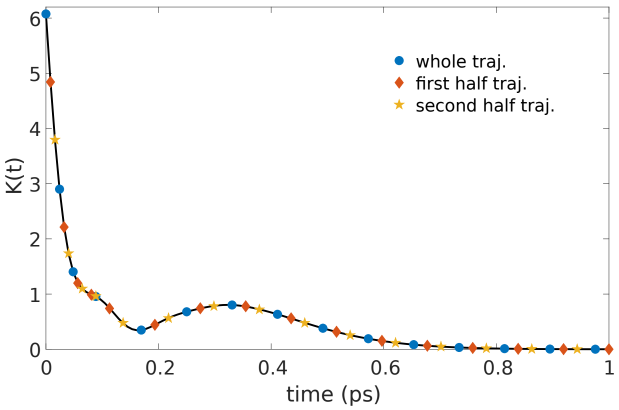


**FIG. 2:** Comparison between the optimised memory kernels $K(t, \tilde{a}, \tilde{\boldsymbol{b}})$, obtained when the whole atomistic MD simulation is employed in the minimisation of the time-non-local effective CG action ("whole traj.", blue circles), and when only the first ("first half traj.", red diamonds) and second half ("second half traj.", yellow stars) of the trajectory are considered. Results from the three setups are indistinguishable on the scale of the figure.

### B. Noise parameter optimisation

In the minimisation workflow described in Sect. IV the noise has been removed by performing its expectation value; at the same time, it must be recovered in order to numerically simulate the GLE of the CG system. In particular, this amounts at determining the parameters $L_j^\alpha$ in Eq. 29, a task that, given the optimised kernel obtained through the solution of Eq. 50 as described in Sec. IV A, can be achieved as follows.

In a rotationally invariant GLE, the memory kernel $K(t)$ is linked to the noise $\boldsymbol{\xi}_I(t)$ by the fluctuation-dissipation theorem (FDT),

$$\langle \xi_I^\alpha(t) \xi_J^\beta(s) \rangle = k_B T K(t-s) \delta^{\alpha\beta} \delta_{IJ}, \qquad (59)$$

where the indexes $I, J = 1, ..., N_B$ run over the CG particles, while $\alpha, \beta = x, y, z$ over the spatial dimensions.

The coloured noise was defined in Eq. 29 as $\xi_{I,n}^\alpha = \sum_{j=1}^M L_j^\alpha\ \eta_{I,n-j}^\alpha$—with $\eta_j^\alpha \in N(0,1)$—so that the discretised version of the FDT in Eq. 59, in the more general case when different kernels $K^\alpha$ are associated to the three spatial directions, can be written as [17]

$$k_B T K_{n-m}^\alpha = \left\langle \sum_{i=1}^M L_i^\alpha \eta_{I,n-i}^\alpha \sum_{j=1}^M L_j^\alpha \eta_{I,m-j}^\alpha \right\rangle =$$
$$= \sum_{i=1}^M \sum_{j=1}^M L_i^\alpha L_j^\alpha \delta_{n-i,m-j}. \qquad (60)$$

For the sake of simplicity we take $m = 0$, so that Eq. 60 simplifies to:

$$k_B T K_n^\alpha = \sum_{i=1}^M \sum_{j=1}^M L_i^\alpha L_j^\alpha \delta_{n-i,-j}, \qquad (61)$$

which, by exploiting the Kronecker delta, can be recast in

$$k_B T K_n^\alpha = \sum_{l=1}^{M-n} L_l^\alpha L_{l+n}^\alpha. \tag{62}$$

Given the kernel $K_n^\alpha$, the value of the $L_l^\alpha$ can now be found by numerically minimising the square of the distance between the left and the right side of Eq. 62 for every $n \in [0, M-1]$, that is [17]:

$$\text{find } \tilde{\boldsymbol{L}}^\alpha : f(\boldsymbol{L}^\alpha) > f(\tilde{\boldsymbol{L}}^\alpha), \quad \forall\, \boldsymbol{L}^\alpha \in \mathbb{R}^M \neq \tilde{\boldsymbol{L}}^\alpha, \tag{63}$$
$$\text{with } f(\boldsymbol{L}^\alpha) = \sum_{n=0}^{M-1} \left( k_B T K_n^\alpha - \sum_{l=1}^{M-n} L_l^\alpha \, L_{l+n}^\alpha \right)^2 .$$

Such a calculation should in principle be done separately for each spatial direction $\alpha = x, y, z$ when the associated $K^\alpha$ are different. At the same time, as discussed in Sec. IV A, in the case of a water system the minimisation of Eq. 50 provided us with optimised kernels that are equal along the three coordinate axes, thus resulting in coefficients $L_l^\alpha$ that are independent on $\alpha$.

## V. DERIVATION OF THE OPTIMIZATION CONSTRAINT ON THE INTEGRAL OF THE MEMORY KERNEL

In applying our method to a water system, we found that introducing the constraints reported in Eqs. 57 and 58 in the minimisation of Eq. 50 was necessary for a regularisation of the memory kernel and of the overall numeric procedure, see discussion in Sec. IV A. We will now focus our attention on the derivation of the constraint in Eq. 57, which relates the integral of the memory kernel to the diffusion coefficient $D$.

The constraint is obtained as follows. We start by recalling the one-dimensional Langevin equation, that is,

$$m\dot{v}(t) = F(t) - \gamma v(t) + \xi(t), \tag{64}$$

where $v(t)$ is the velocity of the particle, $x(t)$ its the position, $m$ its mass, $F(t)$ the external force, $\xi(t)$ a Gaussian white noise and $\gamma$ a dissipation coefficient. If we compare it to the equivalent GLE,

$$m\dot{v}(t) = F(t) - \int_0^t K(t-t')v(t')dt + \tilde{\xi}(t), \tag{65}$$

where $\tilde{\xi}(t)$ is the colored Gaussian noise and $K(t)$ the memory kernel, we can assume that, for times greater than the time-scale on which the memory kernel acts, the following approximation can be introduced [15]:

$$\gamma = \int_0^\infty K(t)dt. \tag{66}$$

We now recall that the diffusion coefficient $D$ is found through the Einstein relation,

$$D = \lim_{t\to\infty} \frac{\langle x(t)^2 \rangle}{2d\, t}, \tag{67}$$

where $d$ is the dimensionality of the space and $\langle x(t)^2 \rangle$ is the mean square displacement. Moreover, we assume that we can use the definition of the diffusion coefficient taken from Brownian motion [4], namely

$$D = \frac{1}{\beta\gamma}, \tag{68}$$

where $\beta = \frac{1}{k_B T}$. Using these relations we can deduce that

$$\gamma = \frac{1}{\beta D} = \int_0^\infty K(t)dt, \tag{69}$$

so that the constraint can therefore be expressed as

$$\tilde{C}_1 = \int_0^\infty K(t)dt - \frac{1}{\beta D} = 0. \tag{70}$$

We here again stress that, despite obtaining at the end of the workflow memory kernels that are equal for the three spatial directions, along the action minimisation procedure we considered the various $K^\alpha$ independent, $\alpha \in \{x, y, z\}$, so that the constraint in Eq. 70 was actually applied in the minimisation of Eq. 50 separately to each of the tree memory kernels. Such a decomposition along the three coordinate axes holds also for the second condition involving the $L_2$ norm of $b(t)$, see Eq. 58 in Sec. IV A and the associated discussion, where we independently constrained the norms of each $b^\alpha(t)$ in constructing the iterative optimisation scheme.

## VI. INTEGRATION ALGORITHMS

The equations of motion for the atomistic case are integrated by the classical Velocity Verlet algorithm. For each spatial component we obtain the following algorithm:

$$v^{n+\frac{1}{2}} = v^n + -\frac{dt}{2m}\nabla U(x^n), \tag{71}$$
$$x^{n+1} = x^n + dt v^{n+\frac{1}{2}}, \tag{72}$$
$$v^{n+1} = v^{n+\frac{1}{2}} - \frac{dt}{2m}\nabla U(x^{n+1}), \tag{73}$$

The equations of motion for the GLE are integrated by an extended form of the Velocity Verlet scheme [17, 18]:

$$v^{n+\frac{1}{2}} = v^n + \frac{dt}{2m}\left(-\nabla U(x^n) - \left(\frac{1}{2}K_1 v^n dt + \sum_{l=n-M+1}^{n-1} K_{n-l+1} v^l dt\right) + \sum_{l=n-M+1}^{n} L_{n-l+1}\eta^l\right), \tag{74}$$

$$x^{n+1} = x^n + dt v^{n+\frac{1}{2}}, \tag{75}$$

$$v^{n+1} = v^{n+\frac{1}{2}} + \frac{dt}{2m}\left(-\nabla U(x^{n+1}) - \left(\frac{1}{2}K_1 v^{n+1} dt + \sum_{l=n-M+2}^{n} K_{n-l+2} v^l dt\right) + \sum_{l=n-M+2}^{n+1} L_{n-l+2}\eta^l\right) \tag{76}$$

where the third line becomes:

$$v^{n+1}(1 + \frac{dt}{2m}^2 K_1) = v^{n+\frac{1}{2}} + \frac{dt}{2m}\left(-\nabla U(x^{n+1}) - \sum_{l=n-M+2}^{n} K_{n-l+2} v^l dt + \sum_{l=n-M+2}^{n+1} L_{n-l+2}\eta^l\right). \tag{77}$$


[1] C. Hijón, P. Español, E. Vanden-Eijnden, and R. Delgado-Buscalioni, Faraday discussions **144**, 301 (2010).

[2] N. Di Pasquale, T. Hudson, and M. Icardi, Physical Review E **99**, 013303 (2019).

[3] S. Nordholm and R. Zwanzig, Journal of Statistical Physics **13**, 347 (1975).

[4] R. Zwanzig, *Nonequilibrium statistical mechanics* (Oxford university press, 2001).

[5] H. Goldstein, C. Poole, and J. Safko, *Classical mechanics* (American Association of Physics Teachers, 2002).

[6] T. Schilling, Physics Reports **972**, 1 (2022).

[7] R. Kubo, Reports on progress in physics **29**, 255 (1966).

[8] L. Ferialdi and A. Bassi, EPL (Europhysics Letters) **98**, 30009 (2012).

[9] E. Walter, *Applied econometric time series fourth edition* (Wiley, 2015).

[10] A. Shapiro, D. Dentcheva, and A. Ruszczynski, *Lectures on stochastic programming: modeling and theory* (SIAM, 2021).

[11] Z. Li, H. S. Lee, E. Darve, and G. E. Karniadakis, The Journal of chemical physics **146**, 014104 (2017).

[12] Y. Yoshimoto, Z. Li, I. Kinefuchi, and G. E. Karniadakis, The Journal of chemical physics **147**, 244110 (2017).

[13] S. Wang, Z. Li, and W. Pan, Soft matter **15**, 7567 (2019).

[14] N. Bockius, J. Shea, G. Jung, F. Schmid, and M. Hanke, Journal of Physics: Condensed Matter **33**, 214003 (2021).

[15] R. Farias, R. O. Ramos, and L. da Silva, Physical Review E **80**, 031143 (2009).

[16] J. A. Nelder and R. Mead, The computer journal **7**, 308 (1965).

[17] Y. Han, J. F. Dama, and G. A. Voth, The Journal of Chemical Physics **149**, 044104 (2018).

[18] H. S. Lee, *Building a Non-Markovian Coarse-Grained Model* (Stanford University, 2018).
